# Supplementary material for: Estimating Approximate Incentive Compatibility
Source: arXiv:1902.09413 source file (2023-12-11)
Supplement: Supplementary file 1 [file appendix_experiments.tex]

\begin{figure}
\centering
\begin{subfigure}{0.47\textwidth}
\includegraphics[width=\linewidth]{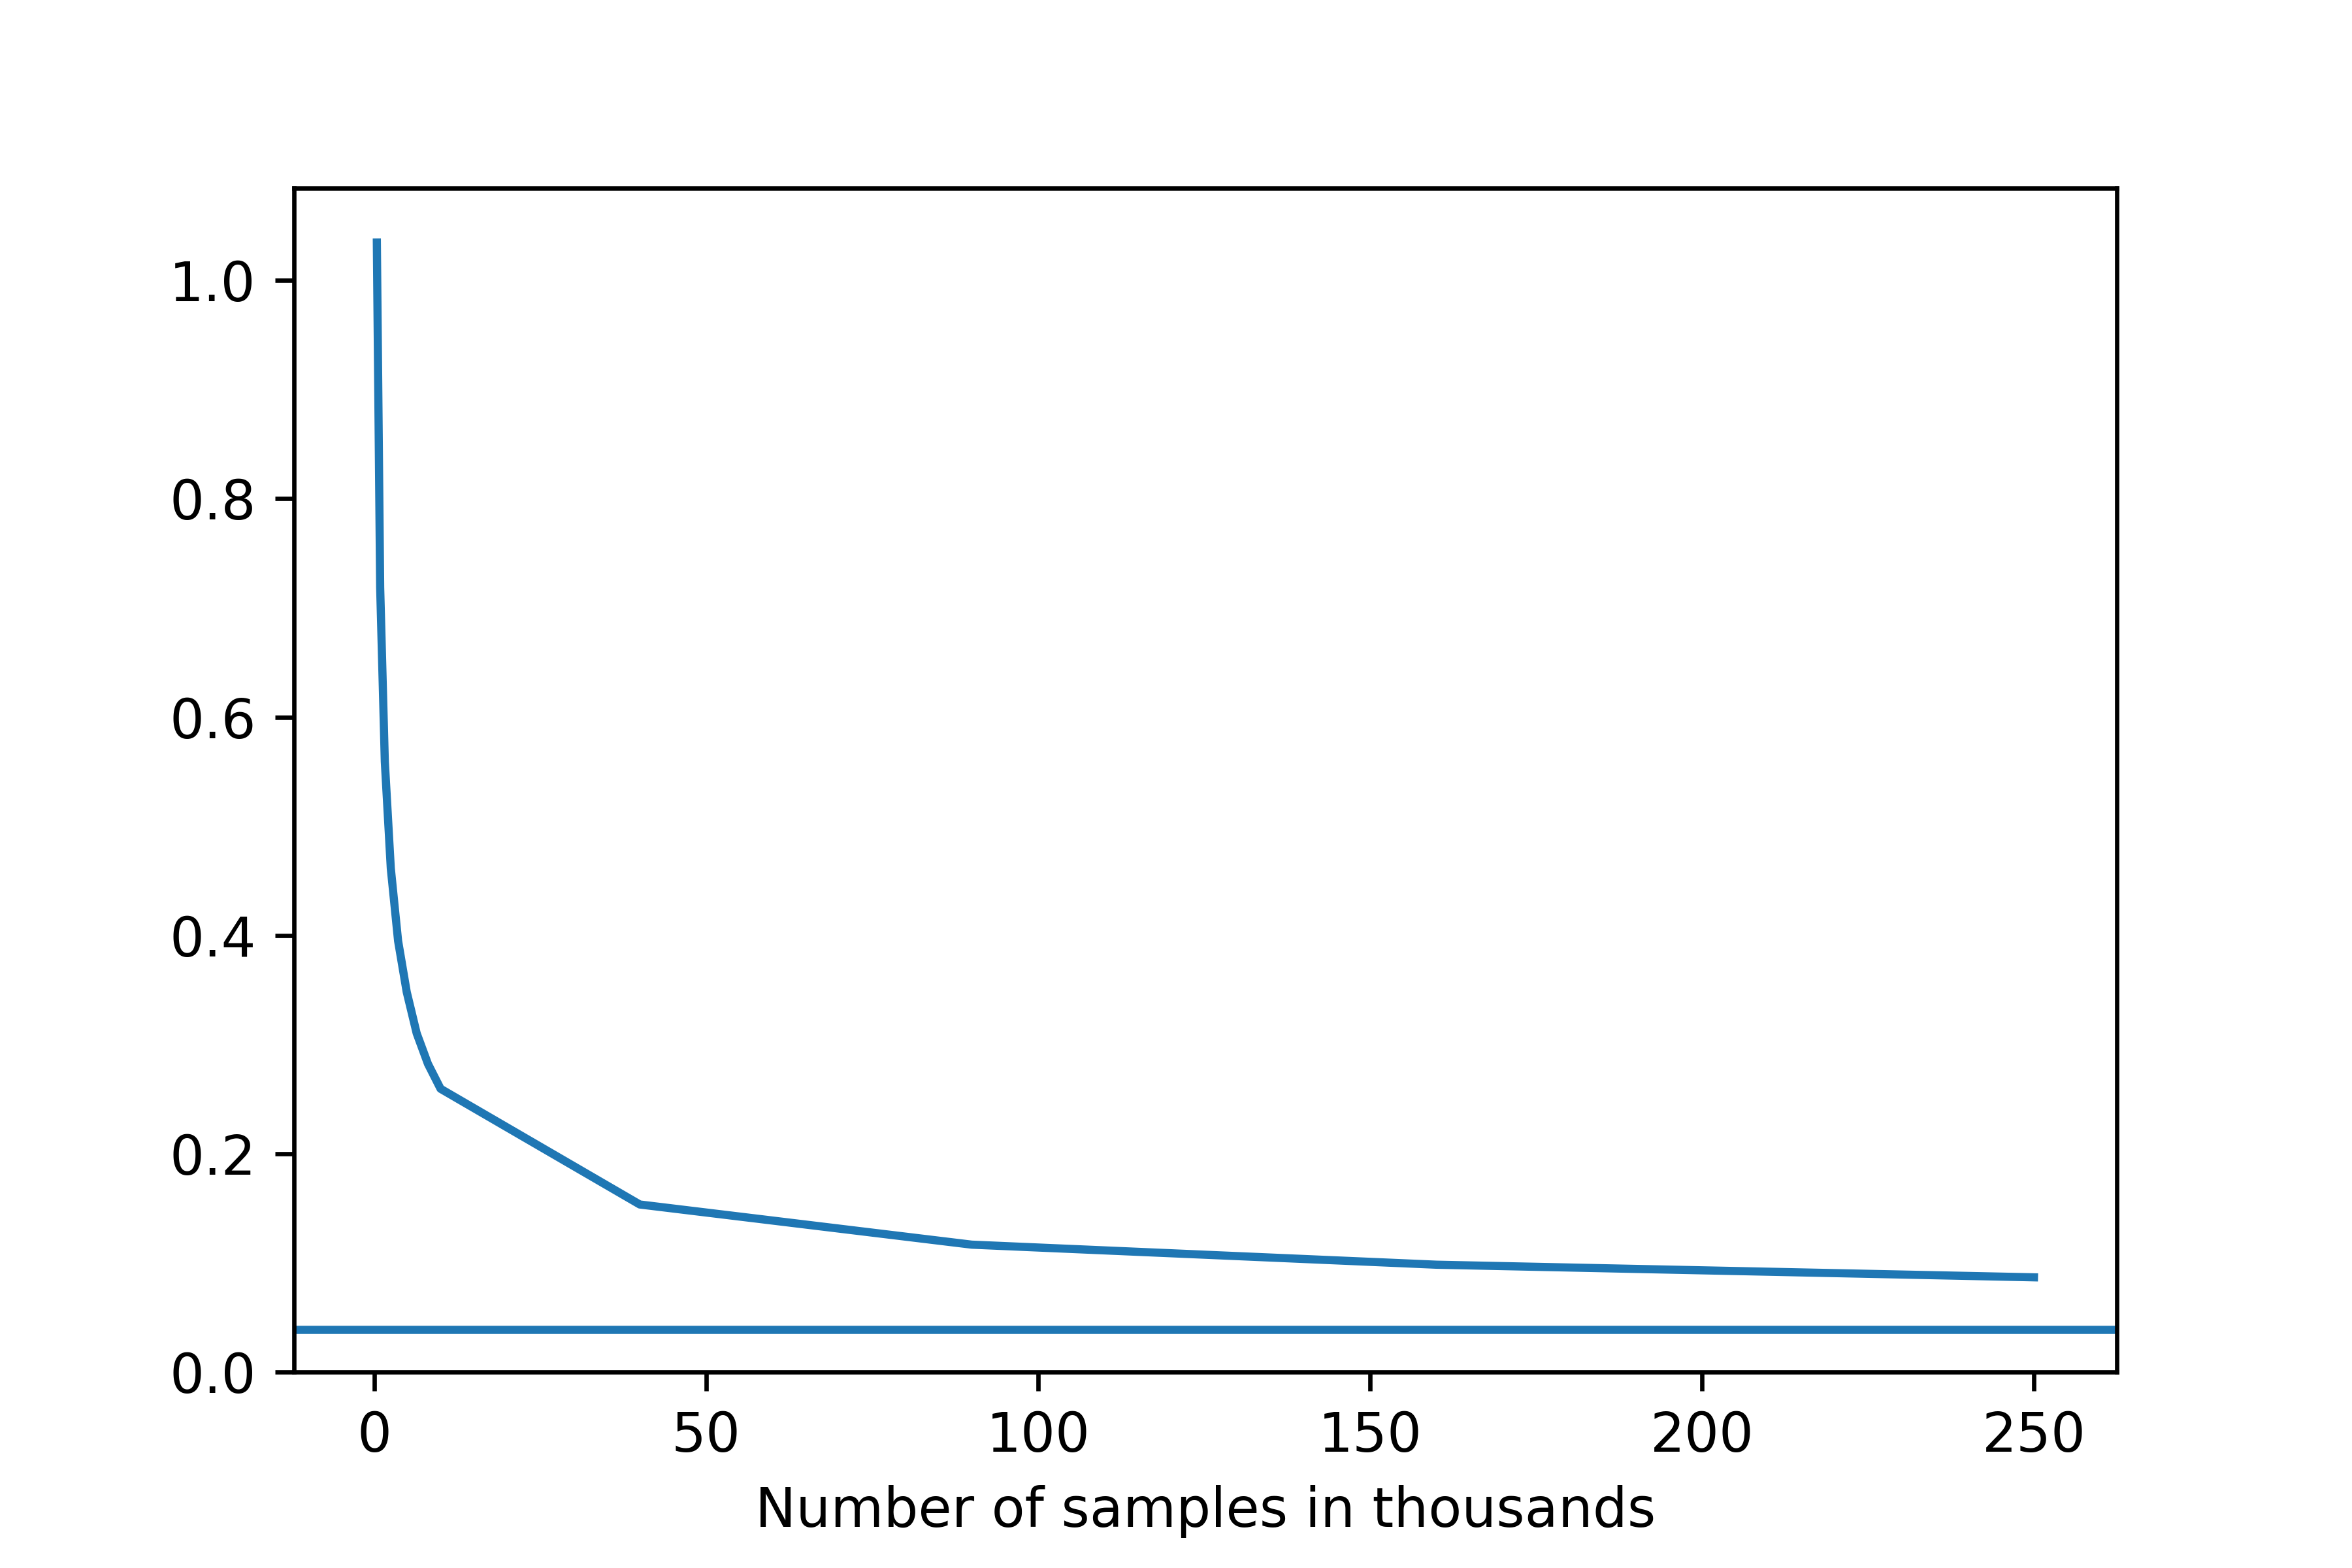} \centering
\caption{First-price auction with 10 bidders.}
\end{subfigure}\qquad
\begin{subfigure}{0.47\textwidth}
\includegraphics[width=\linewidth]{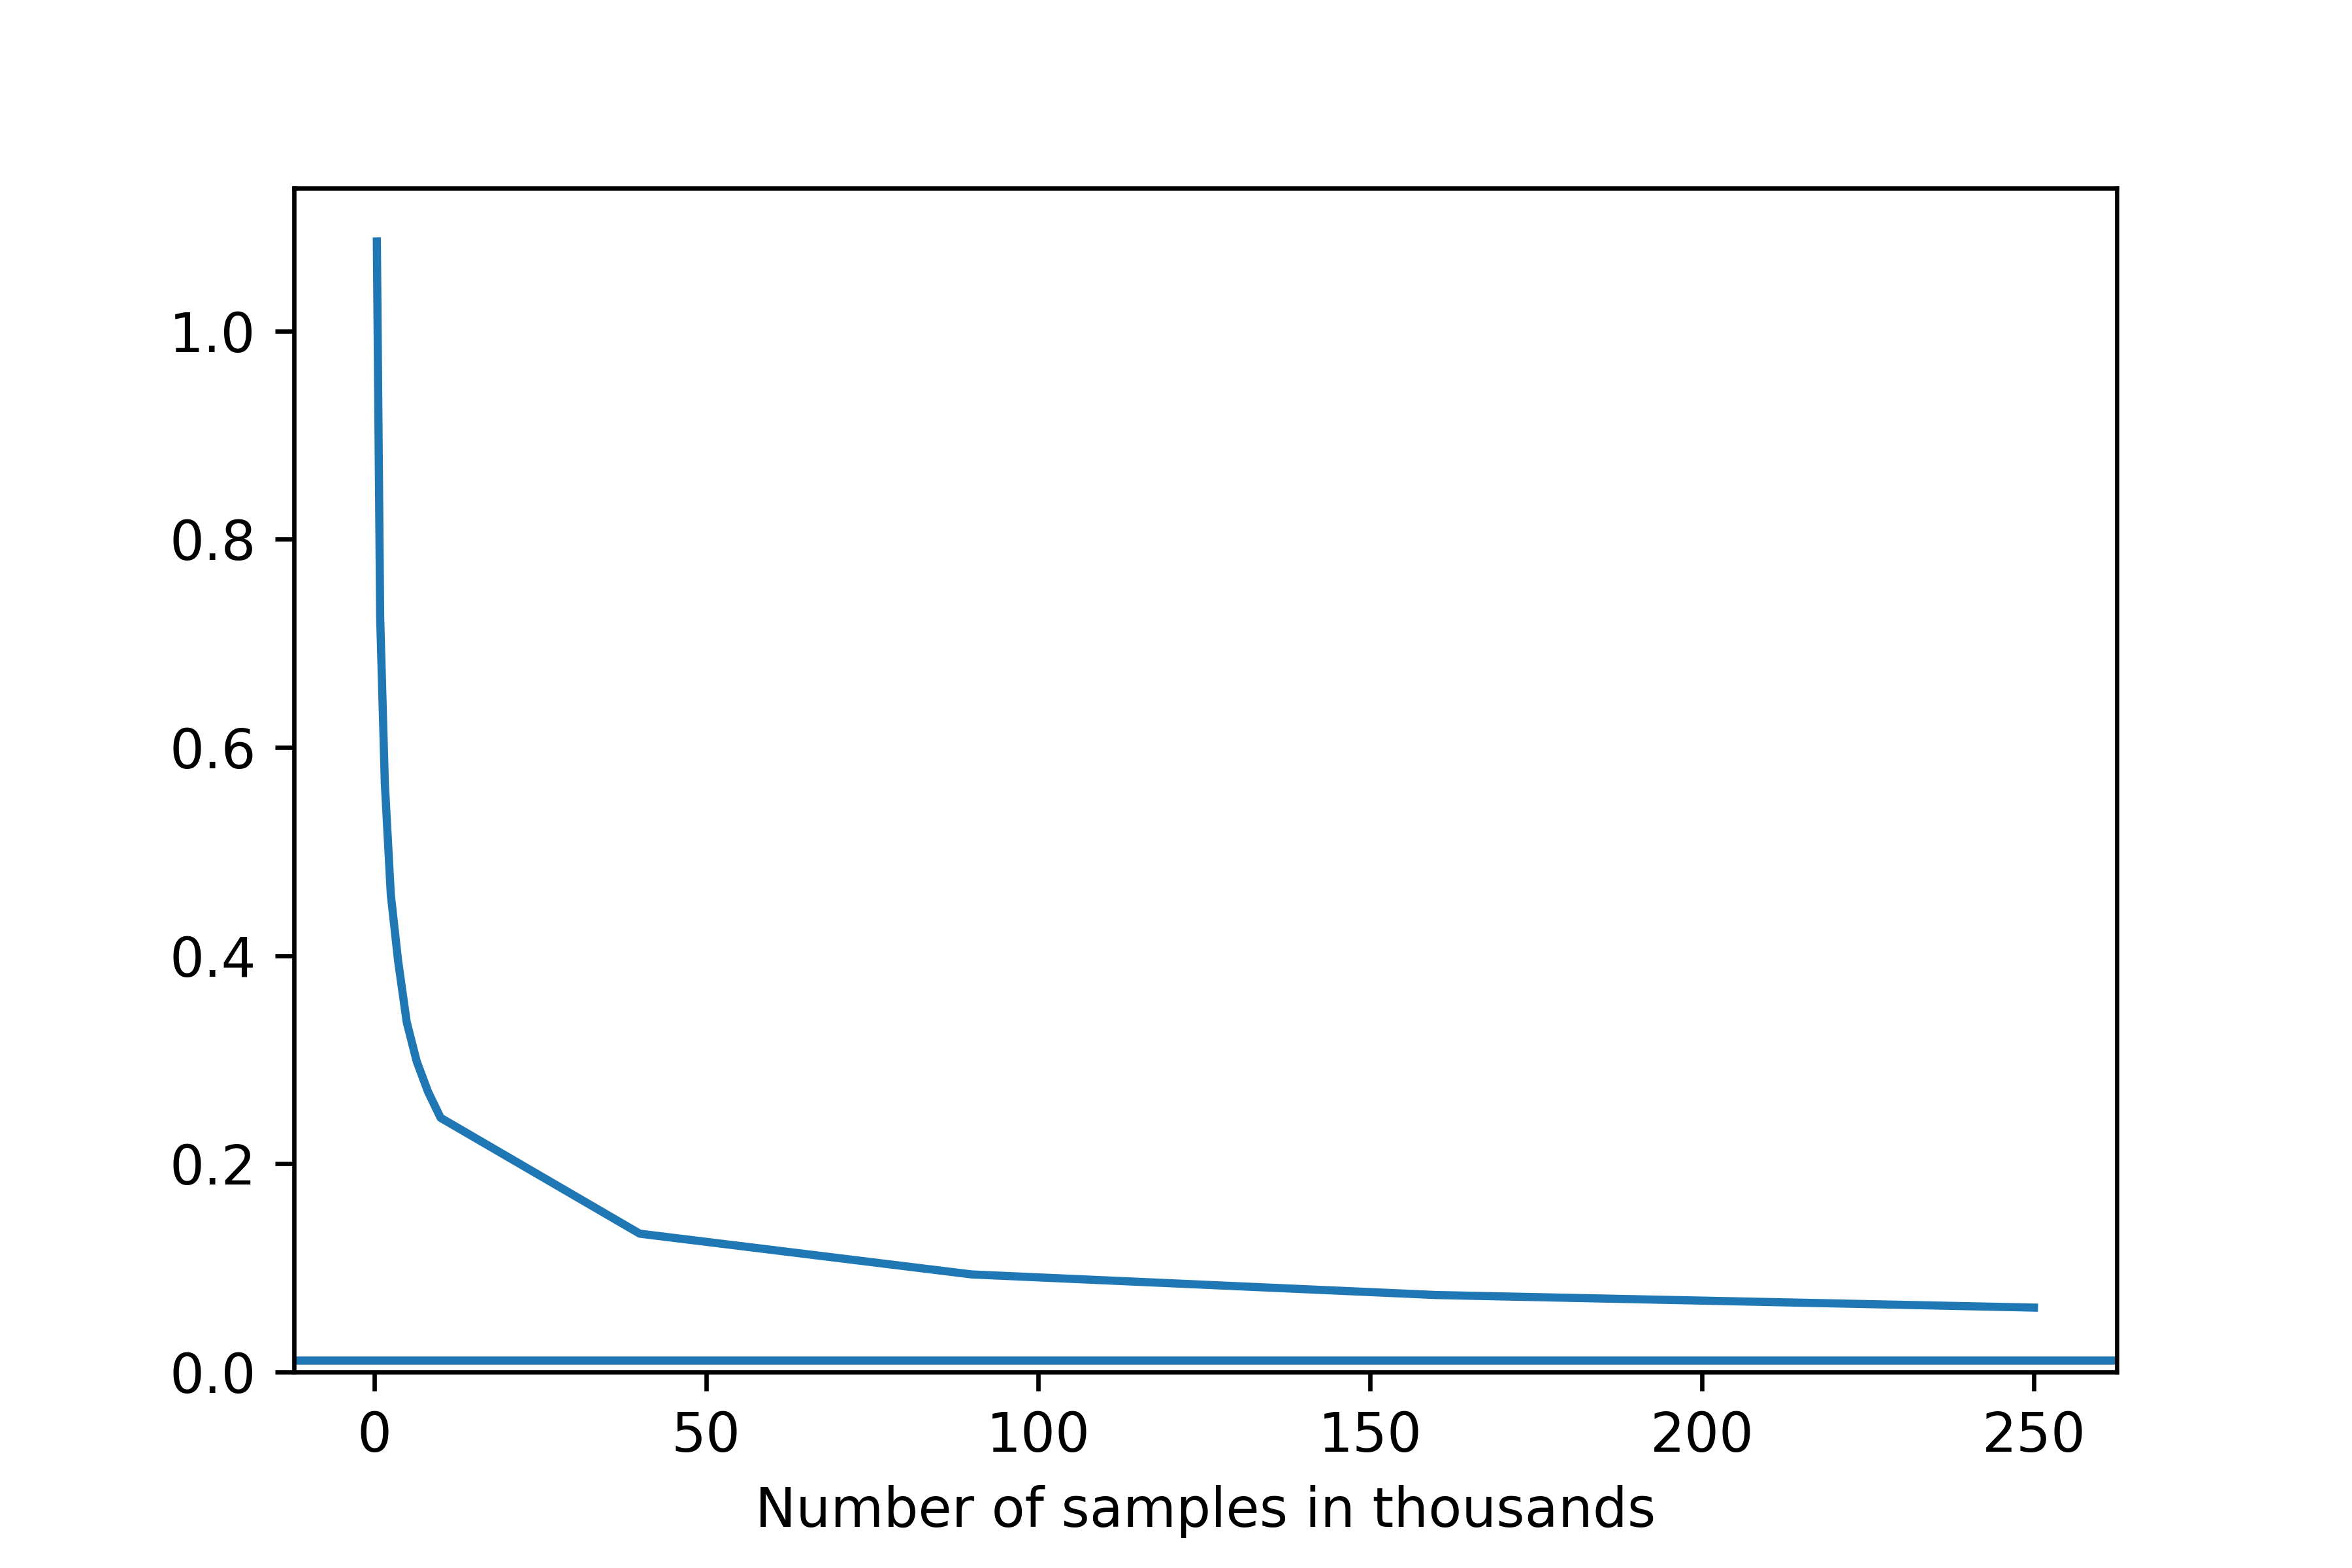}\centering
\caption{Second-price auction with 10 spiteful bidders.}
\end{subfigure}
\caption{Plots illustrating our estimates converging to the true incentive compatibility approximation factors.} 
\label{fig:exp_app}
\end{figure}

We analyze the first-price single-item auction with $n =10$ and the second-price auction with $n =10$, $\alpha_1 = 1/2$, and $\alpha_2 = \alpha_3 = 0$. In both settings, the values are drawn i.i.d. from Uniform(0,1). Under the the first-price auction with $n = 10$, Equation~\eqref{eq:experiments} equals $0.04$. Under the the second-price auction with $n = 10$, Equation~\eqref{eq:experiments} equals $0.01$. These values correspond to the horizontal lines in Figure~\ref{fig:exp_app}.
In all four cases, we range the sample size $N$ up to 250,000 and follow the estimation procedure from Section~\ref{sec:experiments}.
